# Supplementary material for: Quantum critical phase with infinite projected entangled paired states
Source: arXiv:1702.05950 source file (2017-07-14)
Supplement: Supplementary file 1 [file Classification_D=2+2+2+1.pdf]

$\mathbf{S = 1/2,\ n_{occ.} = \{3, 0, 0, 1\}}$

| | | | | | | | | | | | | | | | | |
|---|---|---|---|---|---|---|---|---|---|---|---|---|---|---|---|---|
| State | 1729 | 1730 | 1731 | 1732 | 1733 | 1734 | 1735 | 1736 | 1737 | 1738 | 1739 | 1740 | 1741 | 1742 | 1743 | 1744 |
| Sz | $\frac{1}{2}$ | $-\frac{1}{2}$ | $\frac{1}{2}$ | $-\frac{1}{2}$ | $\frac{1}{2}$ | $-\frac{1}{2}$ | $\frac{1}{2}$ | $-\frac{1}{2}$ | $\frac{1}{2}$ | $-\frac{1}{2}$ | $\frac{1}{2}$ | $-\frac{1}{2}$ | $\frac{1}{2}$ | $-\frac{1}{2}$ | $\frac{1}{2}$ | $-\frac{1}{2}$ |
| Rx | 1 | 1 | 1 | 1 | 0 | 0 | 0 | 0 | 0 | 0 | 0 | 0 | $-1$ | $-1$ | $-1$ | $-1$ |
| Ry | 1 | 1 | 1 | 1 | 0 | 0 | 0 | 0 | 0 | 0 | 0 | 0 | $-1$ | $-1$ | $-1$ | $-1$ |
| R | 1 | 1 | $-1$ | $-1$ | $i$ | $i$ | $i$ | $i$ | $-i$ | $-i$ | $-i$ | $-i$ | 1 | 1 | $-1$ | $-1$ |
| Landau | A1 | A1 | B1 | B1 | E | E | E | E | E | E | E | E | A2 | A2 | B2 | B2 |

$\mathbf{S=1/2,\ n_{occ.}=\{2,1,0,1\}}$

| State | 1745 | 1746 | 1747 | 1748 | 1749 | 1750 | 1751 | 1752 | 1753 | 1754 | 1755 | 1756 | 1757 | 1758 | 1759 | 1760 | 1761 | 1762 | 1763 | 1764 | 1765 | 1766 | 1767 | 1768 |
|---|---|---|---|---|---|---|---|---|---|---|---|---|---|---|---|---|---|---|---|---|---|---|---|---|
| Sz | $\frac{1}{2}$ | $-\frac{1}{2}$ | $\frac{1}{2}$ | $-\frac{1}{2}$ | $\frac{1}{2}$ | $-\frac{1}{2}$ | $\frac{1}{2}$ | $-\frac{1}{2}$ | $\frac{1}{2}$ | $-\frac{1}{2}$ | $\frac{1}{2}$ | $-\frac{1}{2}$ | $\frac{1}{2}$ | $-\frac{1}{2}$ | $\frac{1}{2}$ | $-\frac{1}{2}$ | $\frac{1}{2}$ | $-\frac{1}{2}$ | $\frac{1}{2}$ | $-\frac{1}{2}$ | $\frac{1}{2}$ | $-\frac{1}{2}$ | $\frac{1}{2}$ | $-\frac{1}{2}$ |
| Rx | 1 | 1 | 1 | 1 | 1 | 1 | 1 | 1 | 1 | 1 | 1 | 1 | 0 | 0 | 0 | 0 | 0 | 0 | 0 | 0 | 0 | 0 | 0 | 0 |
| Ry | 1 | 1 | 1 | 1 | 1 | 1 | 1 | 1 | 1 | 1 | 1 | 1 | 0 | 0 | 0 | 0 | 0 | 0 | 0 | 0 | 0 | 0 | 0 | 0 |
| R | 1 | 1 | 1 | 1 | 1 | 1 | $-1$ | $-1$ | $-1$ | $-1$ | $-1$ | $-1$ | $i$ | $i$ | $i$ | $i$ | $i$ | $i$ | $i$ | $i$ | $i$ | $i$ | $i$ | $i$ |
| Landau | A1 | A1 | A1 | A1 | A1 | A1 | B1 | B1 | B1 | B1 | B1 | B1 | E | E | E | E | E | E | E | E | E | E | E | E |

| State | 1769 | 1770 | 1771 | 1772 | 1773 | 1774 | 1775 | 1776 | 1777 | 1778 | 1779 | 1780 | 1781 | 1782 | 1783 | 1784 | 1785 | 1786 | 1787 | 1788 | 1789 | 1790 | 1791 | 1792 |
|---|---|---|---|---|---|---|---|---|---|---|---|---|---|---|---|---|---|---|---|---|---|---|---|---|
| Sz | $\frac{1}{2}$ | $-\frac{1}{2}$ | $\frac{1}{2}$ | $-\frac{1}{2}$ | $\frac{1}{2}$ | $-\frac{1}{2}$ | $\frac{1}{2}$ | $-\frac{1}{2}$ | $\frac{1}{2}$ | $-\frac{1}{2}$ | $\frac{1}{2}$ | $-\frac{1}{2}$ | $\frac{1}{2}$ | $-\frac{1}{2}$ | $\frac{1}{2}$ | $-\frac{1}{2}$ | $\frac{1}{2}$ | $-\frac{1}{2}$ | $\frac{1}{2}$ | $-\frac{1}{2}$ | $\frac{1}{2}$ | $-\frac{1}{2}$ | $\frac{1}{2}$ | $-\frac{1}{2}$ |
| Rx | 0 | 0 | 0 | 0 | 0 | 0 | 0 | 0 | 0 | 0 | 0 | 0 | $-1$ | $-1$ | $-1$ | $-1$ | $-1$ | $-1$ | $-1$ | $-1$ | $-1$ | $-1$ | $-1$ | $-1$ |
| Ry | 0 | 0 | 0 | 0 | 0 | 0 | 0 | 0 | 0 | 0 | 0 | 0 | $-1$ | $-1$ | $-1$ | $-1$ | $-1$ | $-1$ | $-1$ | $-1$ | $-1$ | $-1$ | $-1$ | $-1$ |
| R | $-i$ | $-i$ | $-i$ | $-i$ | $-i$ | $-i$ | $-i$ | $-i$ | $-i$ | $-i$ | $-i$ | $-i$ | 1 | 1 | 1 | 1 | 1 | 1 | $-1$ | $-1$ | $-1$ | $-1$ | $-1$ | $-1$ |
| Landau | E | E | E | E | E | E | E | E | E | E | E | E | A2 | A2 | A2 | A2 | A2 | A2 | B2 | B2 | B2 | B2 | B2 | B2 |

$\mathbf{S = 1/2,\ n_{occ.} = \{2, 0, 1, 1\}}$

| State | 1793 | 1794 | 1795 | 1796 | 1797 | 1798 | 1799 | 1800 | 1801 | 1802 | 1803 | 1804 | 1805 | 1806 | 1807 | 1808 | 1809 | 1810 | 1811 | 1812 | 1813 | 1814 | 1815 | 1816 | 1817 | 1818 | 1819 | 1820 | 1821 | 1822 | 1823 | 1824 | 1825 | 1826 | 1827 | 1828 | 1829 | 1830 | 1831 | 1832 | 1833 | 1834 | 1835 | 1836 | 1837 | 1838 | 1839 | 1840 |
|---|---|---|---|---|---|---|---|---|---|---|---|---|---|---|---|---|---|---|---|---|---|---|---|---|---|---|---|---|---|---|---|---|---|---|---|---|---|---|---|---|---|---|---|---|---|---|---|---|
| Sz | $\frac{1}{2}$ | $-\frac{1}{2}$ | $\frac{1}{2}$ | $-\frac{1}{2}$ | $\frac{1}{2}$ | $-\frac{1}{2}$ | $\frac{1}{2}$ | $-\frac{1}{2}$ | $\frac{1}{2}$ | $-\frac{1}{2}$ | $\frac{1}{2}$ | $-\frac{1}{2}$ | $\frac{1}{2}$ | $-\frac{1}{2}$ | $\frac{1}{2}$ | $-\frac{1}{2}$ | $\frac{1}{2}$ | $-\frac{1}{2}$ | $\frac{1}{2}$ | $-\frac{1}{2}$ | $\frac{1}{2}$ | $-\frac{1}{2}$ | $\frac{1}{2}$ | $-\frac{1}{2}$ | $\frac{1}{2}$ | $-\frac{1}{2}$ | $\frac{1}{2}$ | $-\frac{1}{2}$ | $\frac{1}{2}$ | $-\frac{1}{2}$ | $\frac{1}{2}$ | $-\frac{1}{2}$ | $\frac{1}{2}$ | $-\frac{1}{2}$ | $\frac{1}{2}$ | $-\frac{1}{2}$ | $\frac{1}{2}$ | $-\frac{1}{2}$ | $\frac{1}{2}$ | $-\frac{1}{2}$ | $\frac{1}{2}$ | $-\frac{1}{2}$ | $\frac{1}{2}$ | $-\frac{1}{2}$ | $\frac{1}{2}$ | $-\frac{1}{2}$ | $\frac{1}{2}$ | $-\frac{1}{2}$ |
| Rx | 1 | 1 | 1 | 1 | 1 | 1 | 1 | 1 | 1 | 1 | 1 | 1 | 0 | 0 | 0 | 0 | 0 | 0 | 0 | 0 | 0 | 0 | 0 | 0 | 0 | 0 | 0 | 0 | 0 | 0 | 0 | 0 | 0 | 0 | 0 | 0 | −1 | −1 | −1 | −1 | −1 | −1 | −1 | −1 | −1 | −1 | −1 | −1 |
| Ry | 1 | 1 | 1 | 1 | 1 | 1 | 1 | 1 | 1 | 1 | 1 | 1 | 0 | 0 | 0 | 0 | 0 | 0 | 0 | 0 | 0 | 0 | 0 | 0 | 0 | 0 | 0 | 0 | 0 | 0 | 0 | 0 | 0 | 0 | 0 | 0 | −1 | −1 | −1 | −1 | −1 | −1 | −1 | −1 | −1 | −1 | −1 | −1 |
| R | 1 | 1 | 1 | 1 | 1 | 1 | −1 | −1 | −1 | −1 | −1 | −1 | $i$ | $i$ | $i$ | $i$ | $i$ | $i$ | $i$ | $i$ | $i$ | $i$ | $i$ | $i$ | $-i$ | $-i$ | $-i$ | $-i$ | $-i$ | $-i$ | $-i$ | $-i$ | $-i$ | $-i$ | $-i$ | $-i$ | 1 | 1 | 1 | 1 | 1 | 1 | −1 | −1 | −1 | −1 | −1 | −1 |
| Landau | A1 | A1 | A1 | A1 | A1 | A1 | B1 | B1 | B1 | B1 | B1 | B1 | E | E | E | E | E | E | E | E | E | E | E | E | E | E | E | E | E | E | E | E | E | E | E | E | A2 | A2 | A2 | A2 | A2 | A2 | B2 | B2 | B2 | B2 | B2 | B2 |

$\mathbf{S = 1/2,\ n_{occ.} = \{1, 2, 0, 1\}}$

| State | 1841 | 1842 | 1843 | 1844 | 1845 | 1846 | 1847 | 1848 | 1849 | 1850 | 1851 | 1852 | 1853 | 1854 | 1855 | 1856 |
|---|---|---|---|---|---|---|---|---|---|---|---|---|---|---|---|---|
| Sz | $\frac{1}{2}$ | $-\frac{1}{2}$ | $\frac{1}{2}$ | $-\frac{1}{2}$ | $\frac{1}{2}$ | $-\frac{1}{2}$ | $\frac{1}{2}$ | $-\frac{1}{2}$ | $\frac{1}{2}$ | $-\frac{1}{2}$ | $\frac{1}{2}$ | $-\frac{1}{2}$ | $\frac{1}{2}$ | $-\frac{1}{2}$ | $\frac{1}{2}$ | $-\frac{1}{2}$ |
| Rx | 1 | 1 | 1 | 1 | 1 | 1 | 1 | 1 | 1 | 1 | 1 | 1 | 0 | 0 | 0 | 0 |
| Ry | 1 | 1 | 1 | 1 | 1 | 1 | 1 | 1 | 1 | 1 | 1 | 1 | 0 | 0 | 0 | 0 |
| R | 1 | 1 | 1 | 1 | 1 | 1 | $-1$ | $-1$ | $-1$ | $-1$ | $-1$ | $-1$ | $i$ | $i$ | $i$ | $i$ |
| Landau | A1 | A1 | A1 | A1 | A1 | A1 | B1 | B1 | B1 | B1 | B1 | B1 | E | E | E | E |

| State | 1857 | 1858 | 1859 | 1860 | 1861 | 1862 | 1863 | 1864 | 1865 | 1866 | 1867 | 1868 | 1869 | 1870 | 1871 | 1872 |
|---|---|---|---|---|---|---|---|---|---|---|---|---|---|---|---|---|
| Sz | $\frac{1}{2}$ | $-\frac{1}{2}$ | $\frac{1}{2}$ | $-\frac{1}{2}$ | $\frac{1}{2}$ | $-\frac{1}{2}$ | $\frac{1}{2}$ | $-\frac{1}{2}$ | $\frac{1}{2}$ | $-\frac{1}{2}$ | $\frac{1}{2}$ | $-\frac{1}{2}$ | $\frac{1}{2}$ | $-\frac{1}{2}$ | $\frac{1}{2}$ | $-\frac{1}{2}$ |
| Rx | 0 | 0 | 0 | 0 | 0 | 0 | 0 | 0 | 0 | 0 | 0 | 0 | 0 | 0 | 0 | 0 |
| Ry | 0 | 0 | 0 | 0 | 0 | 0 | 0 | 0 | 0 | 0 | 0 | 0 | 0 | 0 | 0 | 0 |
| R | $i$ | $i$ | $i$ | $i$ | $i$ | $i$ | $i$ | $i$ | $-i$ | $-i$ | $-i$ | $-i$ | $-i$ | $-i$ | $-i$ | $-i$ |
| Landau | E | E | E | E | E | E | E | E | E | E | E | E | E | E | E | E |

| State | 1873 | 1874 | 1875 | 1876 | 1877 | 1878 | 1879 | 1880 | 1881 | 1882 | 1883 | 1884 | 1885 | 1886 | 1887 | 1888 |
|---|---|---|---|---|---|---|---|---|---|---|---|---|---|---|---|---|
| Sz | $\frac{1}{2}$ | $-\frac{1}{2}$ | $\frac{1}{2}$ | $-\frac{1}{2}$ | $\frac{1}{2}$ | $-\frac{1}{2}$ | $\frac{1}{2}$ | $-\frac{1}{2}$ | $\frac{1}{2}$ | $-\frac{1}{2}$ | $\frac{1}{2}$ | $-\frac{1}{2}$ | $\frac{1}{2}$ | $-\frac{1}{2}$ | $\frac{1}{2}$ | $-\frac{1}{2}$ |
| Rx | 0 | 0 | 0 | 0 | $-1$ | $-1$ | $-1$ | $-1$ | $-1$ | $-1$ | $-1$ | $-1$ | $-1$ | $-1$ | $-1$ | $-1$ |
| Ry | 0 | 0 | 0 | 0 | $-1$ | $-1$ | $-1$ | $-1$ | $-1$ | $-1$ | $-1$ | $-1$ | $-1$ | $-1$ | $-1$ | $-1$ |
| R | $-i$ | $-i$ | $-i$ | $-i$ | 1 | 1 | 1 | 1 | 1 | 1 | $-1$ | $-1$ | $-1$ | $-1$ | $-1$ | $-1$ |
| Landau | E | E | E | E | A2 | A2 | A2 | A2 | A2 | A2 | B2 | B2 | B2 | B2 | B2 | B2 |

$\mathbf{S = 1/2}$, $\mathbf{n_{occ.} = \{1, 1, 1, 1\}}$

| State | 1889 | 1890 | 1891 | 1892 | 1893 | 1894 | 1895 | 1896 | 1897 | 1898 | 1899 | 1900 | 1901 | 1902 | 1903 | 1904 | 1905 | 1906 | 1907 | 1908 | 1909 | 1910 | 1911 | 1912 |
|---|---|---|---|---|---|---|---|---|---|---|---|---|---|---|---|---|---|---|---|---|---|---|---|---|
| Sz | $\frac{1}{2}$ | $-\frac{1}{2}$ | $\frac{1}{2}$ | $-\frac{1}{2}$ | $\frac{1}{2}$ | $-\frac{1}{2}$ | $\frac{1}{2}$ | $-\frac{1}{2}$ | $\frac{1}{2}$ | $-\frac{1}{2}$ | $\frac{1}{2}$ | $-\frac{1}{2}$ | $\frac{1}{2}$ | $-\frac{1}{2}$ | $\frac{1}{2}$ | $-\frac{1}{2}$ | $\frac{1}{2}$ | $-\frac{1}{2}$ | $\frac{1}{2}$ | $-\frac{1}{2}$ | $\frac{1}{2}$ | $-\frac{1}{2}$ | $\frac{1}{2}$ | $-\frac{1}{2}$ |
| Rx | 1 | 1 | 1 | 1 | 1 | 1 | 1 | 1 | 1 | 1 | 1 | 1 | 1 | 1 | 1 | 1 | 1 | 1 | 1 | 1 | 1 | 1 | 1 | 1 |
| Ry | 1 | 1 | 1 | 1 | 1 | 1 | 1 | 1 | 1 | 1 | 1 | 1 | 1 | 1 | 1 | 1 | 1 | 1 | 1 | 1 | 1 | 1 | 1 | 1 |
| R | 1 | 1 | 1 | 1 | 1 | 1 | 1 | 1 | 1 | 1 | 1 | 1 | $-1$ | $-1$ | $-1$ | $-1$ | $-1$ | $-1$ | $-1$ | $-1$ | $-1$ | $-1$ | $-1$ | $-1$ |
| Landau | A1 | A1 | A1 | A1 | A1 | A1 | A1 | A1 | A1 | A1 | A1 | A1 | B1 | B1 | B1 | B1 | B1 | B1 | B1 | B1 | B1 | B1 | B1 | B1 |

| State | 1913 | 1914 | 1915 | 1916 | 1917 | 1918 | 1919 | 1920 | 1921 | 1922 | 1923 | 1924 | 1925 | 1926 | 1927 | 1928 | 1929 | 1930 | 1931 | 1932 | 1933 | 1934 | 1935 | 1936 |
|---|---|---|---|---|---|---|---|---|---|---|---|---|---|---|---|---|---|---|---|---|---|---|---|---|
| Sz | $\frac{1}{2}$ | $-\frac{1}{2}$ | $\frac{1}{2}$ | $-\frac{1}{2}$ | $\frac{1}{2}$ | $-\frac{1}{2}$ | $\frac{1}{2}$ | $-\frac{1}{2}$ | $\frac{1}{2}$ | $-\frac{1}{2}$ | $\frac{1}{2}$ | $-\frac{1}{2}$ | $\frac{1}{2}$ | $-\frac{1}{2}$ | $\frac{1}{2}$ | $-\frac{1}{2}$ | $\frac{1}{2}$ | $-\frac{1}{2}$ | $\frac{1}{2}$ | $-\frac{1}{2}$ | $\frac{1}{2}$ | $-\frac{1}{2}$ | $\frac{1}{2}$ | $-\frac{1}{2}$ |
| Rx | 0 | 0 | 0 | 0 | 0 | 0 | 0 | 0 | 0 | 0 | 0 | 0 | 0 | 0 | 0 | 0 | 0 | 0 | 0 | 0 | 0 | 0 | 0 | 0 |
| Ry | 0 | 0 | 0 | 0 | 0 | 0 | 0 | 0 | 0 | 0 | 0 | 0 | 0 | 0 | 0 | 0 | 0 | 0 | 0 | 0 | 0 | 0 | 0 | 0 |
| R | $i$ | $i$ | $i$ | $i$ | $i$ | $i$ | $i$ | $i$ | $i$ | $i$ | $i$ | $i$ | $i$ | $i$ | $i$ | $i$ | $i$ | $i$ | $i$ | $i$ | $i$ | $i$ | $i$ | $i$ |
| Landau | E | E | E | E | E | E | E | E | E | E | E | E | E | E | E | E | E | E | E | E | E | E | E | E |

| State | 1937 | 1938 | 1939 | 1940 | 1941 | 1942 | 1943 | 1944 | 1945 | 1946 | 1947 | 1948 | 1949 | 1950 | 1951 | 1952 | 1953 | 1954 | 1955 | 1956 | 1957 | 1958 | 1959 | 1960 |
|---|---|---|---|---|---|---|---|---|---|---|---|---|---|---|---|---|---|---|---|---|---|---|---|---|
| Sz | $\frac{1}{2}$ | $-\frac{1}{2}$ | $\frac{1}{2}$ | $-\frac{1}{2}$ | $\frac{1}{2}$ | $-\frac{1}{2}$ | $\frac{1}{2}$ | $-\frac{1}{2}$ | $\frac{1}{2}$ | $-\frac{1}{2}$ | $\frac{1}{2}$ | $-\frac{1}{2}$ | $\frac{1}{2}$ | $-\frac{1}{2}$ | $\frac{1}{2}$ | $-\frac{1}{2}$ | $\frac{1}{2}$ | $-\frac{1}{2}$ | $\frac{1}{2}$ | $-\frac{1}{2}$ | $\frac{1}{2}$ | $-\frac{1}{2}$ | $\frac{1}{2}$ | $-\frac{1}{2}$ |
| Rx | 0 | 0 | 0 | 0 | 0 | 0 | 0 | 0 | 0 | 0 | 0 | 0 | 0 | 0 | 0 | 0 | 0 | 0 | 0 | 0 | 0 | 0 | 0 | 0 |
| Ry | 0 | 0 | 0 | 0 | 0 | 0 | 0 | 0 | 0 | 0 | 0 | 0 | 0 | 0 | 0 | 0 | 0 | 0 | 0 | 0 | 0 | 0 | 0 | 0 |
| R | $-i$ | $-i$ | $-i$ | $-i$ | $-i$ | $-i$ | $-i$ | $-i$ | $-i$ | $-i$ | $-i$ | $-i$ | $-i$ | $-i$ | $-i$ | $-i$ | $-i$ | $-i$ | $-i$ | $-i$ | $-i$ | $-i$ | $-i$ | $-i$ |
| Landau | E | E | E | E | E | E | E | E | E | E | E | E | E | E | E | E | E | E | E | E | E | E | E | E |

| State | 1961 | 1962 | 1963 | 1964 | 1965 | 1966 | 1967 | 1968 | 1969 | 1970 | 1971 | 1972 | 1973 | 1974 | 1975 | 1976 | 1977 | 1978 | 1979 | 1980 | 1981 | 1982 | 1983 | 1984 |
|---|---|---|---|---|---|---|---|---|---|---|---|---|---|---|---|---|---|---|---|---|---|---|---|---|
| Sz | $\frac{1}{2}$ | $-\frac{1}{2}$ | $\frac{1}{2}$ | $-\frac{1}{2}$ | $\frac{1}{2}$ | $-\frac{1}{2}$ | $\frac{1}{2}$ | $-\frac{1}{2}$ | $\frac{1}{2}$ | $-\frac{1}{2}$ | $\frac{1}{2}$ | $-\frac{1}{2}$ | $\frac{1}{2}$ | $-\frac{1}{2}$ | $\frac{1}{2}$ | $-\frac{1}{2}$ | $\frac{1}{2}$ | $-\frac{1}{2}$ | $\frac{1}{2}$ | $-\frac{1}{2}$ | $\frac{1}{2}$ | $-\frac{1}{2}$ | $\frac{1}{2}$ | $-\frac{1}{2}$ |
| Rx | $-1$ | $-1$ | $-1$ | $-1$ | $-1$ | $-1$ | $-1$ | $-1$ | $-1$ | $-1$ | $-1$ | $-1$ | $-1$ | $-1$ | $-1$ | $-1$ | $-1$ | $-1$ | $-1$ | $-1$ | $-1$ | $-1$ | $-1$ | $-1$ |
| Ry | $-1$ | $-1$ | $-1$ | $-1$ | $-1$ | $-1$ | $-1$ | $-1$ | $-1$ | $-1$ | $-1$ | $-1$ | $-1$ | $-1$ | $-1$ | $-1$ | $-1$ | $-1$ | $-1$ | $-1$ | $-1$ | $-1$ | $-1$ | $-1$ |
| R | 1 | 1 | 1 | 1 | 1 | 1 | 1 | 1 | 1 | 1 | 1 | 1 | $-1$ | $-1$ | $-1$ | $-1$ | $-1$ | $-1$ | $-1$ | $-1$ | $-1$ | $-1$ | $-1$ | $-1$ |
| Landau | A2 | A2 | A2 | A2 | A2 | A2 | A2 | A2 | A2 | A2 | A2 | A2 | B2 | B2 | B2 | B2 | B2 | B2 | B2 | B2 | B2 | B2 | B2 | B2 |

$\mathbf{S = 1/2,\ n_{occ.} = \{1, 0, 2, 1\}}$

| State | 1985 | 1986 | 1987 | 1988 | 1989 | 1990 | 1991 | 1992 | 1993 | 1994 | 1995 | 1996 | 1997 | 1998 | 1999 | 2000 | 2001 | 2002 | 2003 | 2004 | 2005 | 2006 | 2007 | 2008 |
|---|---|---|---|---|---|---|---|---|---|---|---|---|---|---|---|---|---|---|---|---|---|---|---|---|
| Sz | $\frac{1}{2}$ | $-\frac{1}{2}$ | $\frac{1}{2}$ | $-\frac{1}{2}$ | $\frac{1}{2}$ | $-\frac{1}{2}$ | $\frac{1}{2}$ | $-\frac{1}{2}$ | $\frac{1}{2}$ | $-\frac{1}{2}$ | $\frac{1}{2}$ | $-\frac{1}{2}$ | $\frac{1}{2}$ | $-\frac{1}{2}$ | $\frac{1}{2}$ | $-\frac{1}{2}$ | $\frac{1}{2}$ | $-\frac{1}{2}$ | $\frac{1}{2}$ | $-\frac{1}{2}$ | $\frac{1}{2}$ | $-\frac{1}{2}$ | $\frac{1}{2}$ | $-\frac{1}{2}$ |
| Rx | 1 | 1 | 1 | 1 | 1 | 1 | 1 | 1 | 1 | 1 | 1 | 1 | 0 | 0 | 0 | 0 | 0 | 0 | 0 | 0 | 0 | 0 | 0 | 0 |
| Ry | 1 | 1 | 1 | 1 | 1 | 1 | 1 | 1 | 1 | 1 | 1 | 1 | 0 | 0 | 0 | 0 | 0 | 0 | 0 | 0 | 0 | 0 | 0 | 0 |
| R | 1 | 1 | 1 | 1 | 1 | 1 | $-1$ | $-1$ | $-1$ | $-1$ | $-1$ | $-1$ | $i$ | $i$ | $i$ | $i$ | $i$ | $i$ | $i$ | $i$ | $i$ | $i$ | $i$ | $i$ |
| Landau | A1 | A1 | A1 | A1 | A1 | A1 | B1 | B1 | B1 | B1 | B1 | B1 | E | E | E | E | E | E | E | E | E | E | E | E |

| State | 2009 | 2010 | 2011 | 2012 | 2013 | 2014 | 2015 | 2016 | 2017 | 2018 | 2019 | 2020 | 2021 | 2022 | 2023 | 2024 | 2025 | 2026 | 2027 | 2028 | 2029 | 2030 | 2031 | 2032 |
|---|---|---|---|---|---|---|---|---|---|---|---|---|---|---|---|---|---|---|---|---|---|---|---|---|
| Sz | $\frac{1}{2}$ | $-\frac{1}{2}$ | $\frac{1}{2}$ | $-\frac{1}{2}$ | $\frac{1}{2}$ | $-\frac{1}{2}$ | $\frac{1}{2}$ | $-\frac{1}{2}$ | $\frac{1}{2}$ | $-\frac{1}{2}$ | $\frac{1}{2}$ | $-\frac{1}{2}$ | $\frac{1}{2}$ | $-\frac{1}{2}$ | $\frac{1}{2}$ | $-\frac{1}{2}$ | $\frac{1}{2}$ | $-\frac{1}{2}$ | $\frac{1}{2}$ | $-\frac{1}{2}$ | $\frac{1}{2}$ | $-\frac{1}{2}$ | $\frac{1}{2}$ | $-\frac{1}{2}$ |
| Rx | 0 | 0 | 0 | 0 | 0 | 0 | 0 | 0 | 0 | 0 | 0 | 0 | $-1$ | $-1$ | $-1$ | $-1$ | $-1$ | $-1$ | $-1$ | $-1$ | $-1$ | $-1$ | $-1$ | $-1$ |
| Ry | 0 | 0 | 0 | 0 | 0 | 0 | 0 | 0 | 0 | 0 | 0 | 0 | $-1$ | $-1$ | $-1$ | $-1$ | $-1$ | $-1$ | $-1$ | $-1$ | $-1$ | $-1$ | $-1$ | $-1$ |
| R | $-i$ | $-i$ | $-i$ | $-i$ | $-i$ | $-i$ | $-i$ | $-i$ | $-i$ | $-i$ | $-i$ | $-i$ | 1 | 1 | 1 | 1 | 1 | 1 | $-1$ | $-1$ | $-1$ | $-1$ | $-1$ | $-1$ |
| Landau | E | E | E | E | E | E | E | E | E | E | E | E | A2 | A2 | A2 | A2 | A2 | A2 | B2 | B2 | B2 | B2 | B2 | B2 |

$\mathbf{S = 1/2,\ n_{occ.} = \{1, 0, 0, 3\}}$

$$\left(\begin{array}{ccccccccc} \text{State} & 2033 & 2034 & 2035 & 2036 & 2037 & 2038 & 2039 & 2040 \\ \text{Sz} & \frac{1}{2} & -\frac{1}{2} & \frac{1}{2} & -\frac{1}{2} & \frac{1}{2} & -\frac{1}{2} & \frac{1}{2} & -\frac{1}{2} \\ \text{Rx} & 1 & 1 & 1 & 1 & 0 & 0 & 0 & 0 \\ \text{Ry} & 1 & 1 & 1 & 1 & 0 & 0 & 0 & 0 \\ \text{R} & 1 & 1 & -1 & -1 & i & i & -i & -i \\ \text{Landau} & \text{A1} & \text{A1} & \text{B1} & \text{B1} & \text{E} & \text{E} & \text{E} & \text{E} \end{array}\right)$$

$\mathbf{S = 1/2,\ n_{occ.} = \{0, 3, 0, 1\}}$

| State | 2041 | 2042 | 2043 | 2044 | 2045 | 2046 | 2047 | 2048 | 2049 | 2050 | 2051 | 2052 | 2053 | 2054 | 2055 | 2056 |
|---|---|---|---|---|---|---|---|---|---|---|---|---|---|---|---|---|
| Sz | $\frac{1}{2}$ | $-\frac{1}{2}$ | $\frac{1}{2}$ | $-\frac{1}{2}$ | $\frac{1}{2}$ | $-\frac{1}{2}$ | $\frac{1}{2}$ | $-\frac{1}{2}$ | $\frac{1}{2}$ | $-\frac{1}{2}$ | $\frac{1}{2}$ | $-\frac{1}{2}$ | $\frac{1}{2}$ | $-\frac{1}{2}$ | $\frac{1}{2}$ | $-\frac{1}{2}$ |
| Rx | 1 | 1 | 1 | 1 | 0 | 0 | 0 | 0 | 0 | 0 | 0 | 0 | $-1$ | $-1$ | $-1$ | $-1$ |
| Ry | 1 | 1 | 1 | 1 | 0 | 0 | 0 | 0 | 0 | 0 | 0 | 0 | $-1$ | $-1$ | $-1$ | $-1$ |
| R | 1 | 1 | $-1$ | $-1$ | $i$ | $i$ | $i$ | $i$ | $-i$ | $-i$ | $-i$ | $-i$ | 1 | 1 | $-1$ | $-1$ |
| Landau | A1 | A1 | B1 | B1 | E | E | E | E | E | E | E | E | A2 | A2 | B2 | B2 |

$\mathbf{S = 1/2,\ n_{occ.} = \{0, 2, 1, 1\}}$

| State | 2057 | 2058 | 2059 | 2060 | 2061 | 2062 | 2063 | 2064 | 2065 | 2066 | 2067 | 2068 | 2069 | 2070 | 2071 | 2072 | 2073 | 2074 | 2075 | 2076 | 2077 | 2078 | 2079 | 2080 |
|---|---|---|---|---|---|---|---|---|---|---|---|---|---|---|---|---|---|---|---|---|---|---|---|---|
| Sz | $\frac{1}{2}$ | $-\frac{1}{2}$ | $\frac{1}{2}$ | $-\frac{1}{2}$ | $\frac{1}{2}$ | $-\frac{1}{2}$ | $\frac{1}{2}$ | $-\frac{1}{2}$ | $\frac{1}{2}$ | $-\frac{1}{2}$ | $\frac{1}{2}$ | $-\frac{1}{2}$ | $\frac{1}{2}$ | $-\frac{1}{2}$ | $\frac{1}{2}$ | $-\frac{1}{2}$ | $\frac{1}{2}$ | $-\frac{1}{2}$ | $\frac{1}{2}$ | $-\frac{1}{2}$ | $\frac{1}{2}$ | $-\frac{1}{2}$ | $\frac{1}{2}$ | $-\frac{1}{2}$ |
| Rx | 1 | 1 | 1 | 1 | 1 | 1 | 1 | 1 | 1 | 1 | 1 | 1 | 0 | 0 | 0 | 0 | 0 | 0 | 0 | 0 | 0 | 0 | 0 | 0 |
| Ry | 1 | 1 | 1 | 1 | 1 | 1 | 1 | 1 | 1 | 1 | 1 | 1 | 0 | 0 | 0 | 0 | 0 | 0 | 0 | 0 | 0 | 0 | 0 | 0 |
| R | 1 | 1 | 1 | 1 | 1 | 1 | $-1$ | $-1$ | $-1$ | $-1$ | $-1$ | $-1$ | $i$ | $i$ | $i$ | $i$ | $i$ | $i$ | $i$ | $i$ | $i$ | $i$ | $i$ | $i$ |
| Landau | A1 | A1 | A1 | A1 | A1 | A1 | B1 | B1 | B1 | B1 | B1 | B1 | E | E | E | E | E | E | E | E | E | E | E | E |

| State | 2081 | 2082 | 2083 | 2084 | 2085 | 2086 | 2087 | 2088 | 2089 | 2090 | 2091 | 2092 | 2093 | 2094 | 2095 | 2096 | 2097 | 2098 | 2099 | 2100 | 2101 | 2102 | 2103 | 2104 |
|---|---|---|---|---|---|---|---|---|---|---|---|---|---|---|---|---|---|---|---|---|---|---|---|---|
| Sz | $\frac{1}{2}$ | $-\frac{1}{2}$ | $\frac{1}{2}$ | $-\frac{1}{2}$ | $\frac{1}{2}$ | $-\frac{1}{2}$ | $\frac{1}{2}$ | $-\frac{1}{2}$ | $\frac{1}{2}$ | $-\frac{1}{2}$ | $\frac{1}{2}$ | $-\frac{1}{2}$ | $\frac{1}{2}$ | $-\frac{1}{2}$ | $\frac{1}{2}$ | $-\frac{1}{2}$ | $\frac{1}{2}$ | $-\frac{1}{2}$ | $\frac{1}{2}$ | $-\frac{1}{2}$ | $\frac{1}{2}$ | $-\frac{1}{2}$ | $\frac{1}{2}$ | $-\frac{1}{2}$ |
| Rx | 0 | 0 | 0 | 0 | 0 | 0 | 0 | 0 | 0 | 0 | 0 | 0 | $-1$ | $-1$ | $-1$ | $-1$ | $-1$ | $-1$ | $-1$ | $-1$ | $-1$ | $-1$ | $-1$ | $-1$ |
| Ry | 0 | 0 | 0 | 0 | 0 | 0 | 0 | 0 | 0 | 0 | 0 | 0 | $-1$ | $-1$ | $-1$ | $-1$ | $-1$ | $-1$ | $-1$ | $-1$ | $-1$ | $-1$ | $-1$ | $-1$ |
| R | $-i$ | $-i$ | $-i$ | $-i$ | $-i$ | $-i$ | $-i$ | $-i$ | $-i$ | $-i$ | $-i$ | $-i$ | 1 | 1 | 1 | 1 | 1 | 1 | $-1$ | $-1$ | $-1$ | $-1$ | $-1$ | $-1$ |
| Landau | E | E | E | E | E | E | E | E | E | E | E | E | A2 | A2 | A2 | A2 | A2 | A2 | B2 | B2 | B2 | B2 | B2 | B2 |

$\mathbf{S = 1/2,\ n_{occ.} = \{0, 1, 2, 1\}}$

| State | 2105 | 2106 | 2107 | 2108 | 2109 | 2110 | 2111 | 2112 | 2113 | 2114 | 2115 | 2116 | 2117 | 2118 | 2119 | 2120 | 2121 | 2122 | 2123 | 2124 | 2125 | 2126 | 2127 | 2128 |
|---|---|---|---|---|---|---|---|---|---|---|---|---|---|---|---|---|---|---|---|---|---|---|---|---|
| Sz | $\frac{1}{2}$ | $-\frac{1}{2}$ | $\frac{1}{2}$ | $-\frac{1}{2}$ | $\frac{1}{2}$ | $-\frac{1}{2}$ | $\frac{1}{2}$ | $-\frac{1}{2}$ | $\frac{1}{2}$ | $-\frac{1}{2}$ | $\frac{1}{2}$ | $-\frac{1}{2}$ | $\frac{1}{2}$ | $-\frac{1}{2}$ | $\frac{1}{2}$ | $-\frac{1}{2}$ | $\frac{1}{2}$ | $-\frac{1}{2}$ | $\frac{1}{2}$ | $-\frac{1}{2}$ | $\frac{1}{2}$ | $-\frac{1}{2}$ | $\frac{1}{2}$ | $-\frac{1}{2}$ |
| Rx | 1 | 1 | 1 | 1 | 1 | 1 | 1 | 1 | 1 | 1 | 1 | 1 | 0 | 0 | 0 | 0 | 0 | 0 | 0 | 0 | 0 | 0 | 0 | 0 |
| Ry | 1 | 1 | 1 | 1 | 1 | 1 | 1 | 1 | 1 | 1 | 1 | 1 | 0 | 0 | 0 | 0 | 0 | 0 | 0 | 0 | 0 | 0 | 0 | 0 |
| R | 1 | 1 | 1 | 1 | 1 | 1 | −1 | −1 | −1 | −1 | −1 | −1 | $i$ | $i$ | $i$ | $i$ | $i$ | $i$ | $i$ | $i$ | $i$ | $i$ | $i$ | $i$ |
| Landau | A1 | A1 | A1 | A1 | A1 | A1 | B1 | B1 | B1 | B1 | B1 | B1 | E | E | E | E | E | E | E | E | E | E | E | E |

| State | 2129 | 2130 | 2131 | 2132 | 2133 | 2134 | 2135 | 2136 | 2137 | 2138 | 2139 | 2140 | 2141 | 2142 | 2143 | 2144 | 2145 | 2146 | 2147 | 2148 | 2149 | 2150 | 2151 | 2152 |
|---|---|---|---|---|---|---|---|---|---|---|---|---|---|---|---|---|---|---|---|---|---|---|---|---|
| Sz | $\frac{1}{2}$ | $-\frac{1}{2}$ | $\frac{1}{2}$ | $-\frac{1}{2}$ | $\frac{1}{2}$ | $-\frac{1}{2}$ | $\frac{1}{2}$ | $-\frac{1}{2}$ | $\frac{1}{2}$ | $-\frac{1}{2}$ | $\frac{1}{2}$ | $-\frac{1}{2}$ | $\frac{1}{2}$ | $-\frac{1}{2}$ | $\frac{1}{2}$ | $-\frac{1}{2}$ | $\frac{1}{2}$ | $-\frac{1}{2}$ | $\frac{1}{2}$ | $-\frac{1}{2}$ | $\frac{1}{2}$ | $-\frac{1}{2}$ | $\frac{1}{2}$ | $-\frac{1}{2}$ |
| Rx | 0 | 0 | 0 | 0 | 0 | 0 | 0 | 0 | 0 | 0 | 0 | 0 | −1 | −1 | −1 | −1 | −1 | −1 | −1 | −1 | −1 | −1 | −1 | −1 |
| Ry | 0 | 0 | 0 | 0 | 0 | 0 | 0 | 0 | 0 | 0 | 0 | 0 | −1 | −1 | −1 | −1 | −1 | −1 | −1 | −1 | −1 | −1 | −1 | −1 |
| R | $-i$ | $-i$ | $-i$ | $-i$ | $-i$ | $-i$ | $-i$ | $-i$ | $-i$ | $-i$ | $-i$ | $-i$ | 1 | 1 | 1 | 1 | 1 | 1 | −1 | −1 | −1 | −1 | −1 | −1 |
| Landau | E | E | E | E | E | E | E | E | E | E | E | E | A2 | A2 | A2 | A2 | A2 | A2 | B2 | B2 | B2 | B2 | B2 | B2 |

$\mathbf{S = 1/2,\ n_{occ.} = \{0, 1, 0, 3\}}$

$$\left(\begin{array}{ccccccccc} \text{State} & 2153 & 2154 & 2155 & 2156 & 2157 & 2158 & 2159 & 2160 \\ \text{Sz} & \frac{1}{2} & -\frac{1}{2} & \frac{1}{2} & -\frac{1}{2} & \frac{1}{2} & -\frac{1}{2} & \frac{1}{2} & -\frac{1}{2} \\ \text{Rx} & 1 & 1 & 1 & 1 & 0 & 0 & 0 & 0 \\ \text{Ry} & 1 & 1 & 1 & 1 & 0 & 0 & 0 & 0 \\ \text{R} & 1 & 1 & -1 & -1 & i & i & -i & -i \\ \text{Landau} & \text{A1} & \text{A1} & \text{B1} & \text{B1} & \text{E} & \text{E} & \text{E} & \text{E} \end{array}\right)$$

$\mathbf{S = 1/2,\ n_{occ.} = \{0, 0, 3, 1\}}$

| State | 2161 | 2162 | 2163 | 2164 | 2165 | 2166 | 2167 | 2168 | 2169 | 2170 | 2171 | 2172 | 2173 | 2174 | 2175 | 2176 |
|---|---|---|---|---|---|---|---|---|---|---|---|---|---|---|---|---|
| Sz | $\frac{1}{2}$ | $-\frac{1}{2}$ | $\frac{1}{2}$ | $-\frac{1}{2}$ | $\frac{1}{2}$ | $-\frac{1}{2}$ | $\frac{1}{2}$ | $-\frac{1}{2}$ | $\frac{1}{2}$ | $-\frac{1}{2}$ | $\frac{1}{2}$ | $-\frac{1}{2}$ | $\frac{1}{2}$ | $-\frac{1}{2}$ | $\frac{1}{2}$ | $-\frac{1}{2}$ |
| Rx | 1 | 1 | 1 | 1 | 0 | 0 | 0 | 0 | 0 | 0 | 0 | 0 | $-1$ | $-1$ | $-1$ | $-1$ |
| Ry | 1 | 1 | 1 | 1 | 0 | 0 | 0 | 0 | 0 | 0 | 0 | 0 | $-1$ | $-1$ | $-1$ | $-1$ |
| R | 1 | 1 | $-1$ | $-1$ | $i$ | $i$ | $i$ | $i$ | $-i$ | $-i$ | $-i$ | $-i$ | 1 | 1 | $-1$ | $-1$ |
| Landau | A1 | A1 | B1 | B1 | E | E | E | E | E | E | E | E | A2 | A2 | B2 | B2 |

$\mathbf{S = 1/2,\ n_{occ.} = \{0, 0, 1, 3\}}$

$$\left(\begin{array}{ccccccccc} \text{State} & 2177 & 2178 & 2179 & 2180 & 2181 & 2182 & 2183 & 2184 \\ \text{Sz} & \frac{1}{2} & -\frac{1}{2} & \frac{1}{2} & -\frac{1}{2} & \frac{1}{2} & -\frac{1}{2} & \frac{1}{2} & -\frac{1}{2} \\ \text{Rx} & 1 & 1 & 1 & 1 & 0 & 0 & 0 & 0 \\ \text{Ry} & 1 & 1 & 1 & 1 & 0 & 0 & 0 & 0 \\ \text{R} & 1 & 1 & -1 & -1 & i & i & -i & -i \\ \text{Landau} & \text{A1} & \text{A1} & \text{B1} & \text{B1} & \text{E} & \text{E} & \text{E} & \text{E} \end{array}\right)$$
